# Supplementary material for: Rapid behavioral transitions produce chaotic mixing by a planktonic microswimmer
Source: arXiv:1804.08773 source file (2018-04-23)
Supplement: Supplementary file 1 [file blinking_paper_arxiv_supps2.pdf]

# Contents

**1 Supplementary Figures** **25**

**2 Supplementary Videos** **27**

**3 Supplementary Methods** **29**

A Experimental techniques and data analysis . . . . . . . . . . . . . . . . . . . . 29

B Theoretical model FTLE Analysis . . . . . . . . . . . . . . . . . . . . . . . . . 35

C Simulations of feeding in theoretical model . . . . . . . . . . . . . . . . . . . 37

# 1 Supplementary Figures

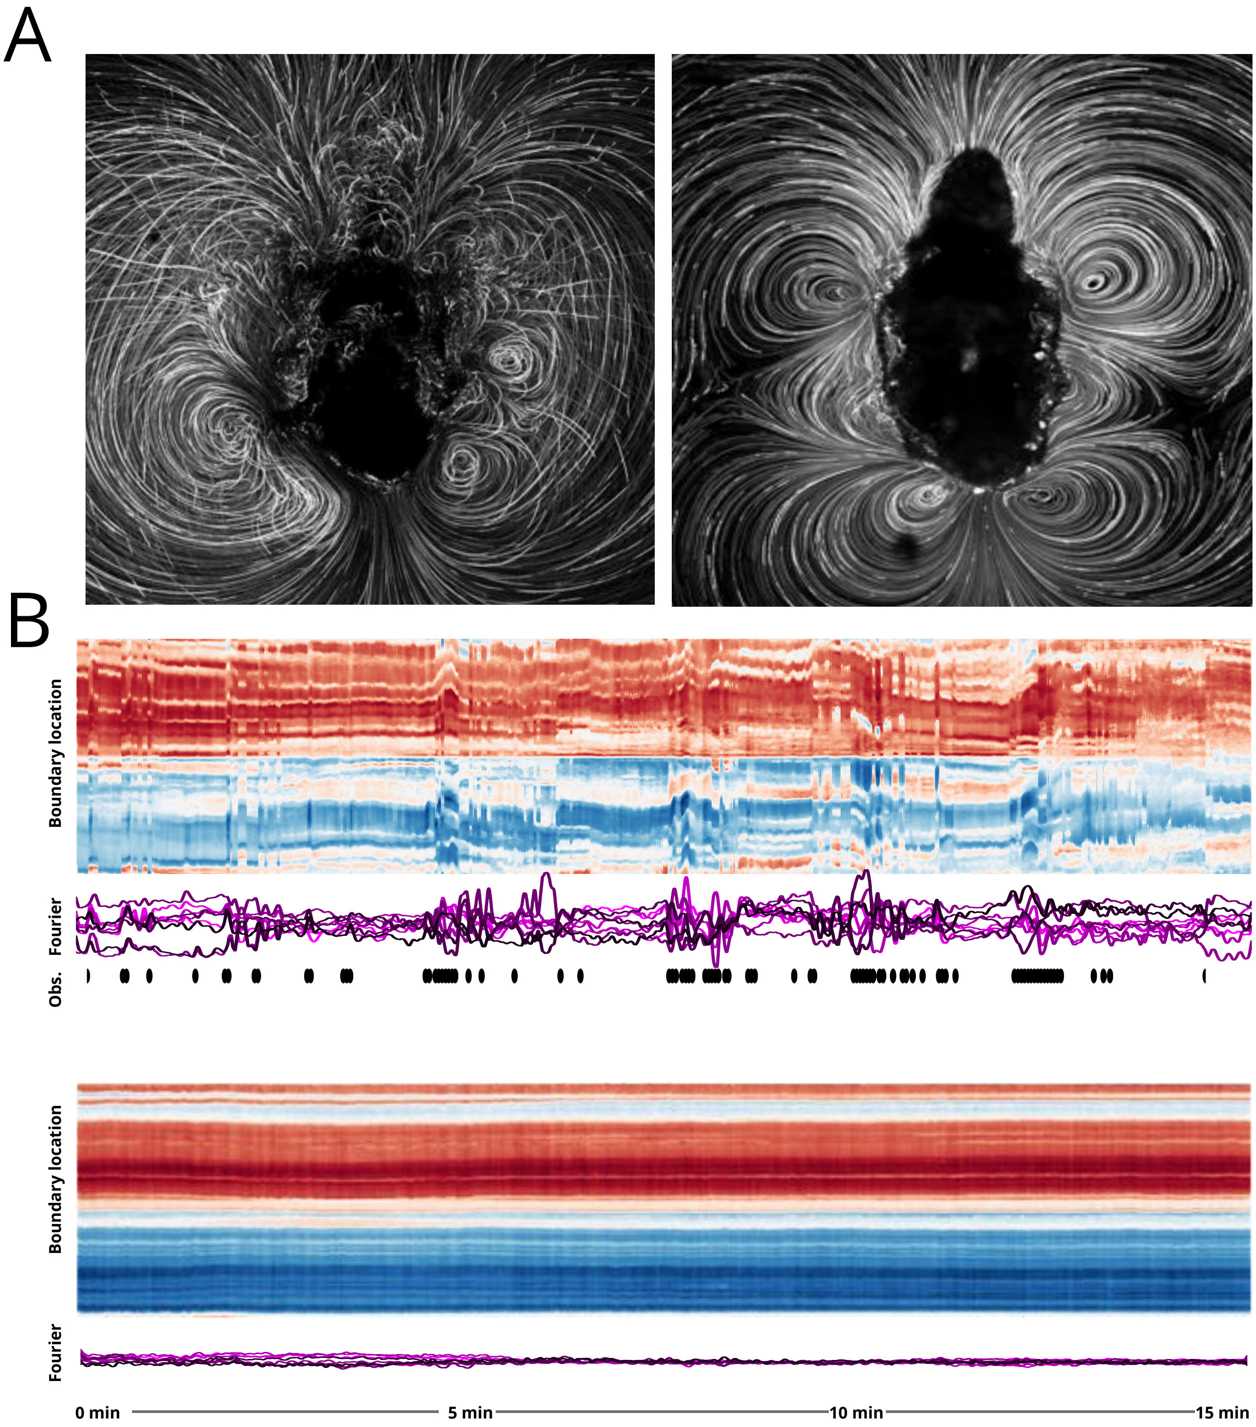


**Figure S1 Response of larva to treatment with $MgCl_2$.** (A) A 60 second timelapse of 2 $\mu$m fluorescent particles advected by starfish larvae immobilized beneath a cover slip, before (left) and after (right) incubation in $MgCl_2$. (B) Boundary condition kymographs and best-fit Fourier coefficients for example 15 minute videos before (top) and after (bottom) treatment.

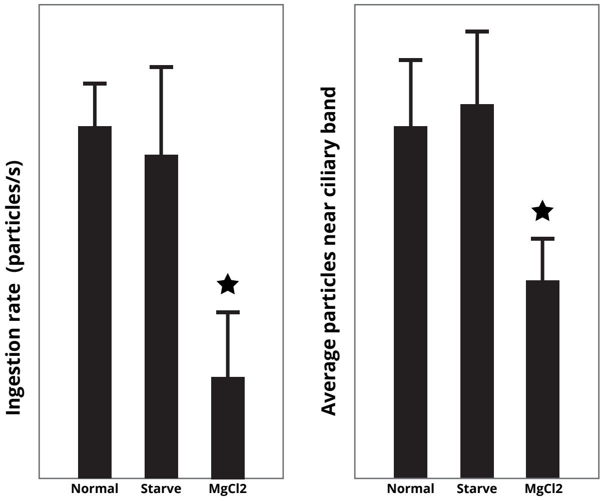


**Figure S2 Effect of $MgCl_2$ and starvation on larval feeding rates** The left bars show the relative amount of new particles arriving in the mouth and stomach region, representing ingestion. The right bars show the relative amount of particles contacting the ciliary band, on average. Significance established using Welch's. 13 animals from the laboratory culture were used for the "Normal" treatment, 14 animals treated with $MgCl_2$ were used for the "$MgCl_2$" treatment, and 13 animals starved for one week were used for the "Starve" treatment. Error bars correspond to standard deviations, and significance asterisk corresponds to Welch's test with $p < 0.01$.

# 2 Supplementary Videos

**SI Video 1.** A real-time video of a blinking transition, with frames stacked over a 1.5 second interval in order to visualize the motion of 0.75 $\mu$m particles in the water. Field of view is 3.3 mm.

**SI Video 2.** A 25x speed video of blinking during a 15 minute video, with frames stacked over a 18 second interval in order to visualize the motion of 0.75 $\mu$m particles in the water. Field of view is 3.3 mm.

**SI Video 3.** A real time video of the ciliary band during a blinking event. Field of view is 700 $\mu$m.

**SI Video 4.** A real time video of the ciliary band and algae particle capture during a blinking event. Field of view is 700 $\mu$m.

**SI Video 5.** A real time video of the ciliary band and algae particle capture during a blinking event. Field of view is 460 $\mu$m

**SI Video 6.** An 8x speed video of 2 $\mu$m yellow-green fluorescent particles around a larva under fluorescence illumination. Frames stacked over 60 s in order to visualize trajectories. Field of view is 3.3 mm.

**SI Video 7.** An 8x speed video of 2 $\mu$m yellow-green fluorescent particles around an $MgCl_2$-treated larva under fluorescence illumination. Frames stacked over 60 s in order to visualize trajectories. Field of view is 3.3 mm.

**SI Video 8.** A real-time video of two $MgCl_2$-treated larvae colliding while freely swimming in a Petri dish. Field of view is 5.5 mm.

**SI Video 9.** An 8x speed video of ingestion of 6 $\mu$m tracer particles by a larva. Field of view is 1.4 mm.

**SI Video 10.** An 8x speed video of ingestion of 6 $\mu$m tracer particles by an $MgCl_2$-treated larva. Note that the bolus of particles in the stomach predates drug treatment, and the drug inhibits the larval ability to further digest these pre-existing trapped particles. Field of view is 1.4 mm.

**SI Video 11.** Video of the distortion of a cloud of particles by a squirmer undergoing a single "blink" event, with timescales and boundary conditions set by the mean values of the experimental datasets.

**SI Video 12.** A short-time simulation of the distortion of a "stripe" of particles by a model squirmer during a blinking event.

# 3 Supplementary Methods

## A Experimental techniques and data analysis

**Spawning and culturing larval starfish.** Adult samples of *Patiria miniata* were collected by the Monterey Abalone Company, based in Monterey, CA. Animals were placed in plastic bins containing filtered sea water from Monterey Bay, and allowed to equilibrate overnight. Spawning was induced by injecting the gonopores of gravid adults with 1-methyadenine. For males, dry sperm was collected using a transfer pipette, and then diluted by a factor of 10. Female adults were rarer and successfully spawned less often, but once eggs first started to appear on the surface of an adult female, the animal was inverted over a 500 mL beaker to facilitate egg collection. Eggs were collected for roughly 30 minutes, and then 8 drops of the diluted sperm was added to the beaker. Embryos were then placed in flat bottom casserole dishes, and they developed and reached their first swimming stages within 5 days. Morphometrics and development parameters for the spawned larvae, as well as temperature control and incubation procedures, are described in further detail in our previous work.[4]

Upon reaching swimming stages, the animals were fed an equal mixture of the phytoplankton *Dunaliella tertiolecta* and *Rhodomonas lens* every four days. Culture water was filtered and replaced every week. At the one-week stage, filtered natural seawater was substituted with osmotically-matched artificial sea water, in order to ensure reproducibility. Before all experiments, water was filtered again with a 1 $\mu$m syringe filter to remove algae clumps.

**Magnesium chloride treatment.** For behavioral inhibition assays, a 50% mixture of artificial salt water and 7.5% $MgCl_2$ solution was prepared and then diluted until the salinity matched that of the artificial sea water stock. Larvae were placed in a Petri dish containing this solution for 30 minutes, and then imaged.

**Acquisition of experimental images**. Animals were imaged using a Nikon TE2000-U microscope and an ORCAFlash4.0 camera under dark field illumination conditions, which

minimizes excess heat and light exposure. Most videos were taken at 20 fps, and the faster playback rate of videos included with this manuscript was set by deleting alternate frames when necessary. For the particle image velocimetry measurements used to generate behavioral kymographs, neutrally-buoyant 0.75 $\mu$m beads (Polysciences) were mixed into artificial sea water at a dilution of 1 : 500 from the stock. During long imaging time series (15 minutes), excess cold water was kept on the slide in order to avoid temperature drift over time. After acquisition, the images were checked using automated scripts to detect evidence of systematic drift in the flow fields over time, and no clear patterns emerged that would suggest satiation, strain, or other long-term consequences of immobilization on the behavior. Larvae were returned to a separate culture after imaging, and the culture of post-experiment animals did not display any noticeable pattern of developmental irregularity or mortality relative to the stock larval culture.

**Velocity field data analysis.** The experimental videos were converted into $67 \times 67$ px velocity fields using the open-source Python package openPIV (http://www.openpiv.net/openpiv-python/). No masking was performed on the swimmer body, in order to avoid artificial edge effects on the boundary. Instead, for each raw image the coordinates of the boundary of the starfish were extracted and ordered by their coordinates along the arclength. The relative angular position $\theta$ at each point on the boundary then recorded, as was the local curvature. For a given angular arc of fixed length, the relative length of the segment of the boundary contained within it measures the degree to which the boundary is either distorted due to strong curvature, or oblique relative to the direction $\hat{\boldsymbol{\theta}}$. In order to account for the former case, for fixed-with bins along $\theta$ weights were assigned to each point on the boundary based on inversely on the local curvature. Then, using the velocity field generated by the PIV code for the same image, the expected velocity vector at each boundary point was calculated. Finally, for each angular bin the weighted average velocity vector for all boundary points within that bin was calculated. The goal of this boundary-reweighing technique is to partly decouple spatial patterns in the boundary conditions due to

the animal's morphology from patterns arising from underlying dynamics of the ciliary band, which facilitates easier comparison of the boundary conditions across animals with distinct morphologies. However, for classifying characteristic features in the boundary conditions, or identifying the locations of sign changes or other noteworthy features on the boundary, the unweighted boundary conditions returned by the raw PIV analysis are sufficient. Across all datasets, we find that the resulting angular velocity distribution, $\mathbf{v}(\theta)$, exhibits the expected property $\mathbf{v}(\theta) \cdot \hat{\boldsymbol{\theta}} \gg \mathbf{v}(\theta) \cdot \hat{\mathbf{r}}$, indicating that the no-flux boundary condition is preserved in the 2D flow field analysis. This allows a single time dependent field, $v_\theta(\theta, t)$ to be used to summarize the larval behavior, resulting in the two-dimensional behavioral kymographs shown in the main text.

**Determination of typical behavioral modes using principal component analysis (PCA).** For the simulations of feeding rates under various conditions, we sought to classify a set of "typical" flow fields around the swimmer that are indicative of the blinking versus steady swimming behaviors. For each animal dataset, we computed leading-order, time-dependent series coefficients of the boundary conditions, $\mathbf{B}(t) = B_1(t), B_2(t), ...$ The amplitudes of the Fourier coefficients $B_k(t)$ decrease with $k$ due to the limited minimal spatial scale at which larvae can control boundary conditions on their surface; for the analysis here, we used the first $M = 10$ Fourier coefficients, but almost identical results emerge when we use $M = 25$ or $M = 50$ coefficients. If there are $N$ frames in a video (and thus $N$ samples of the boundary conditions), we create an $M \times N$ matrix of features and samples (timepoints). We whiten and then perform PCA on this matrix using the Python package scikit-learn (`http://scikit-learn.org/`). Across all datasets, the eigenvalue spectrum of the PC shows a strong ($\sim$ 60%) dropoff after the first two eigenvalues, consistent with the boundary conditions at any given timepoint consisting of a linear superposition of two characteristic behavioral modes. We then project the whitened data matrix onto these two principal components, and threshold the resulting $2 \times N$ time series to classify each of the $N$ frames as belonging to the first or the second principal component. We then return to the

original dataset, and average frames belonging to each class in order to generate estimates of $\mathbf{B}_{swim}$ and $\mathbf{B}_{blink}$. For the simulations, these two typical behavioral modes were averaged across all animals studied.

We note that executing the analysis in the opposite order—performing PCA on the full boundary velocity profile data, and then taking the Fourier transform of the resulting principal components in order to yield $B^i_{swim}, B^i_{blink}$ values—does not strongly affect the observed flow fields, although it does introduce additional noise into the principal component eigenvalue spectrum. Additionally, we note that the general structure and timing of the two modes that we report is strongly independent of the specific clustering algorithm applied; similar results are obtained by using similar manifold learning algorithms to PCA (such as ICA or LDA). Additionally, we found that fitting the behavioral data to a hidden Markov model using the open-source package hmmlearn (`http://hmmlearn.readthedocs.io`) yielded similar results, but with relatively low fit confidence.

**Experimental determination of duty cycle $\nu$ and blinking time $T$.** For a given animal behavior dataset, the power spectra of all of the time-dependent Fourier sine coefficients $c_n(t)$ were calculated and averaged. The first peak in the resulting power spectrum occurs at $1/T_{swim}$, and thus provides the overall timescale of behavioral changes. Error bars are determined by the standard deviation of the averaged power spectrum for each individual. The duty cycle is determined from the average duration of blinks determined by algorithmically classifying the two states in the behavioral time series through PCA (as described above), and then calculating the average contiguous period that the animal spends in each mode. The leading order timescale in both analyses corresponds to events identifiable as "blinks" in the experimental videos.

**Experimental determination of particle capture from fluorescence data.** Fluorescence feeding experiments were performed using 2 $\mu$m yellow-green fluorescent particles, diluted into artificial sea water with a ratio of 1:500. Bead solution was homogenized with a vortex mixer, and then mixed with filtered water from an algae stock culture. Larvae were

immobilized in droplets under cover slips, and the bead mixture was then injected under coverslip until it had displaced the fluid from the original droplet. Larvae were allowed one minute to stabilize before imaging.

Five minute videos at 20 fps (6000 frames) were taken for multiple larvae under each experimental condition. The fluorescence videos readily show clear differences in the uptake of fluorescent particles under various treatment conditions. In order to quantify this effect, each video was first processed using particle image velocimetry in order to estimate the velocity field near the larval surface. This velocity field was then used to bin the spatial regions in each frame of the original video, in order to identify the capture regions near the larval surface.

The boundary of the larvae was extracted from still photos, and the total fluorescence within 30 $\mu$m of the surface (a typical ciliary length) was recorded in each frame and then divided by the average fluorescence of single particles (isolated via image analysis) in the video. As a secondary check, for randomly chosen datasets the total number of particles visible near the band was manually counted and averaged over subsequences of frames, and the total number was found to be consistent with the fluorescence measurements. The number of particles within this interception distance was averaged across all frames in a movie in order to produce an estimate of the total capture opportunities during the dataset, and the distribution of these times across different organisms was used to generate error bars.

In order to estimate the total particles that actually enter the mouth and digestive system (the clearance rate), a region of interest corresponding to the mouth and stomach was manually selected, and total integrated fluorescence intensity in this region was calculated, and the slope of this curve was taken as a proxy for ingestion rate. Occasional muscular events (peristaltic contractions, regurgitation, and defecation) cause occasional rapid changes in the integrated intensity in this region, and so these portions of each video were manually inspected and removed. As a secondary check, higher magnification videos (such as those

shown in the supplementary videos) were used in which the stomach was focus isolated, allowing single particle arrivals to be manually counted and compared to the fluorescence data.

**Confinement effects in experimental data sets.** Due to the small length scales and fast timescales involved in the starfish flow dynamics, long-term animal tracking and light sheet imaging are infeasible in our system. As a result, we immobilize our larvae between two cover slips. The cover slip spacing 500 $\mu$m is not sufficient to induce Hele-Shaw flow in the near field that we study, however it does induce a global recirculation in the flow field due to water pushed past the surface by the swimming stroke eventually reaching a boundary. To leading order, we may compensate for this effect by subtracting a Stokeslet from the velocity field, in order to account for missing drag on the immobilized swimmer's body.[40] At larger distances from the larval body, more sophisticated models are necessary, such as image force singularities that account for slide spacing effects[21] and asymptotic connection of the velocity field to an explicit squirmer model under the Brinkmann approximation.[41] However, here we limit ourselves to studying the feeding currents within 1-2 body lengths of the larva.

We note that in our previous work on starfish larvae,[4] we compared the confined flow fields to the instantaneous velocities of freely-swimming larvae in the Supplementary Material and found general agreement near the surface. Other workers have investigated the effect of instead immobilizing animals using a tether (a suction pipette affixed to the larval surface, permitting imaging without any nearby walls);[19, 20, 42] however, this technique does not remove the leading-order dipole contribution to the flow field, and we have found it induces behavioral irregularities due to high pressures and torques acting on the larval surface at the pipette contact point.

Importantly, for all behavior analysis here, we use the velocity field at the boundary to compute all fluid dynamical quantities of interest. Due to the relative small size of cilia $\approx 30$ $\mu$m compared to the slide spacing $\approx 500$ $\mu$m, we expect negligible mechanical feedback on

ciliary operation.

**Experimental FTLE Analysis.** Particle image velocimetry (PIV) data was taken at a frame rate of 20 fps and frame size of $2048 \times 2048$ px. For each FTLE calculation, a subsample of 100 consecutive frames 5 s centered to a randomly-chosen blinking event was chosen for each animal and used for further study. Bash scripts were used to rename PIV files as $0001.txt, 0002.txt, ...,$ with the data stored in each file formatted into four tab-delimited columns $x \quad y \quad vx \quad vy$. After this pre-processing, the PIV data sets were ready for use with the LCS MATLAB Kit v1.0 (http://dabirilab.com/software/).[27]

Within the LCS Kit, the PIV data was processed using the parameter set: forward FTLE, integration length 100 frames, time interval $0.05s$, step size 1 frame, window size $2048 \times 2048$ px, mesh size $101 \times 101$ px. Due to substructure in the experimental velocity field on scales smaller than the PIV mesh size $< 10\mu m$, the fluid incompressibility equation is not locally satisfied at all points in the experimental velocity field, leading to negative largest FTLE values in regions of the velocity field containing strong velocity gradients or local circulation. When analyzing the FTLE spectral properties, these values were discarded; empirically, they tend to occur in low-velocity regions far from the swimmer's body, rather than in the complex near-field regions that contribute predominantly to mixing.

The unnormalized distribution of finite-time Lyapunov exponents, $F(\lambda_t)$, was calculated directly from the values outputted of the LCS Kit, and dimensionalized accordingly based on the pixel resolution and frame rate.

## B Theoretical model FTLE Analysis

For the theoretical model, a dense mesh of points around the squirmer model body was initialized. The motion of these points subject to the model's time-varying velocity field was computed for a given integration time $T$ by defining the flow map, $\phi$, over that integration

time. The maximal FTLE field is then computed as a function of space using the equation

$$\lambda(\mathbf{r}) \equiv \frac{1}{\tau} \max \left[ \mathrm{eig} \left( \log \left( \frac{d\phi_0^\tau(\mathbf{r})}{d\mathbf{r}} \right) \right) \right].$$

In order to characterize the flow, we primarily focus on the FTLE spectrum induced by single behavioral transitions. Much of the literature on blinking vortex maps and periodic turbulent flows analyzes the effect of repeated iterations of a chaotic map on the FTLE spectrum.[25, 29, 30, 43] However, in our system we find that the general shape of the FTLE distribution is invariant under repeated behavioral transitions, with the shape and width of the FTLE distribution being related to the number of completed blinking cycles by a trivial rescaling. Moreover, a real-world larva would not have uniform inter-blink intervals, making some phenomena that occur in chaotic maps with uniform period duration (such as fractal-like geometric arrangements of advected particles) less applicable to our system.

Instead, here we perform simulations of length $T$, in which the swimmer stays within the swimming behavioral mode for $t = 0$ to $t = T/2$, and then instantaneously transitions into the blinking mode for $t = T/2$ to $t = T$. As $T$ varies, the form and structure of the FTLE field varies appreciably, as is visible in Figure S3.

**Analysis of mixing using the FTLE spectrum.** We apply recent results that relate the explicit form of the spectrum of maximal FTLE to the expected power spectrum of a passive scalar advected by a flow. We are particularly concerned with results related to mixing properties of turbulent and chaotic flows that apply above the "diffusive cutoff" because the trajectories of the 5-25 $\mu$m algae particles typically ingested by the larvae display negligible diffusivity over timescales relevant to their interaction with the larva.

The following results are derived by Antonsen et al.[30, 44] and Fereday et al.[31] For a periodic chaotic flow, the power spectrum of a passive scalar $F(k, t)$ is related to the distribution

of finite time Lyapunov exponents $P(\lambda, t)$ by the relation,

$$F(k,t) \approx \frac{1}{k\,t} P\left(t^{-1}\log\frac{k}{k_0}, t\right)$$

where $k_0$ is the wavenumber at which the passive scalar is injected. We assume here that $k_0 \ll 1$, or that spatial variation in the algae field encountered by the swimmer occurs over scales much larger than the swimmer's body. We convert the distribution of FTLE values provided by the data or model analysis to a spatial spectrum using the identity

$$F(k,t) = \int P(\lambda,t)\delta(k - k_0\exp(\lambda\, t))\; d\lambda.$$

In our system, this power spectrum is observed to have the form $F(k,t) \sim k^{-3}$ for both the experimental data and the theoretical model of a swimmer in an open flow (Figure 4C in the main text). The same scaling is observed in simulations of two-dimensional turbulence at high Schmidt number,[32, 45] suggesting that this scaling is consistent with behavioral fluctuations producing a "forward cascade" in the distribution of particles advected by the fluid field around the body. We verify that this process affects feeding dynamics across time by observing that the mean of $F(k,t)$, $\bar{k}(t)$, gradually increases in time, consistent with "filamentation" occurring in the local flow field due to inhomogeneities in the local nutrient field being stretched to smaller and smaller length scales.[46, 47] This process is visible at long timescales in Figure S3.

## C Simulations of feeding in theoretical model

The general approach behind our feeding rate calculations is based on analysis of pathlines of advected particles under the time-varying flow field produced by the swimmer. We define a finite "interception radius" around the swimmer, which we set as a value equivalent to one ciliary length in the experimental data. However, as long as the interception radius is sufficiently small, the total capture rate will trivially scale linearly with this parameter.

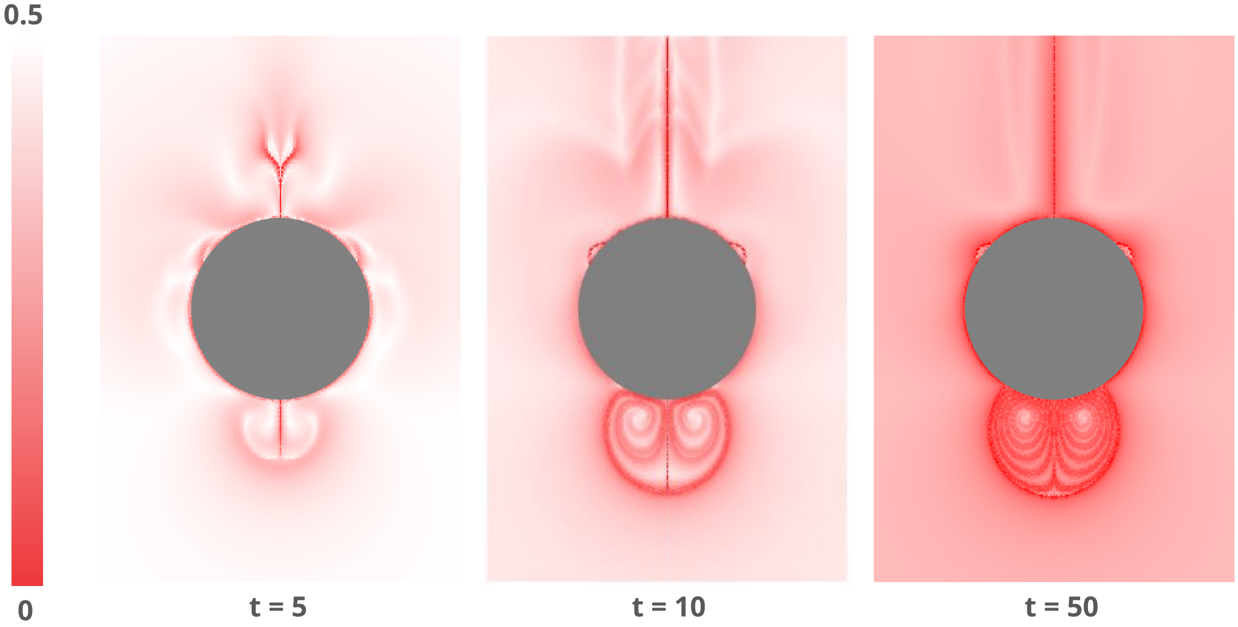


**Figure S3 Development of coherent structures in the blinking flow field.** The field of finite-time Lyaponov exponents (FTLE) around the swimmer as a function of integration time.

We then calculate the trajectories of large numbers of particles in the far field that the swimmer approaches and encounters, and then analyze the number of particles that enter the interception region, and the duration of time that they spend there.

The concept of an interception radius, and its functional consequences for feeding versus swimming, has previously been explored for other marine organisms and zooplankton,[48, 49] revealing unique fluid dynamical mechanisms of prey ambush and particle size selection based on distinct behavioral strategies.[13, 50, 51] Here, we are particularly interested in how the continuous and dynamics boundary conditions afforded by a ciliary band affect the time dynamics of particle encounter rates.

Because most algae ingested by the larvae are larger than 2 $\mu$m and swim at speeds much lower than the $\sim$ 500 $\mu$m maximum speeds near the ciliary band,[4] we observe negligible streamline crossing effects in the near field due to diffusion either via Brownian motion or active swimming by entrained algae. Inertial effects due to Stokes' drift are also negligible at this small length scale and low Reynolds' number, and so the feeding mechanism of the

starfish larvae operates in a distinct regime from other planktonic filter feeders that modulate particle encounter rates though flow regime control mechanisms.[52, 53]

**Determination of the far field starting distance.** In order to determine the effective starting distance for particle capture simulations and other components of the analysis, a criterion for the far-field starting distance, $x_{par}$, must be defined. At this distance away from the swimmer, food particles travel along effectively parallel streamlines in the commoving frame of the swimmer.

A simple heuristic for determining the distance $x_{par}$ is to define the maximum shear in the velocity field as a function of $x_{par}$,

$$a(x_{par}) \equiv \max_y \left( \frac{\partial v_x}{\partial y}\bigg|_{x_{par}} \right)$$
$$b(x_{par}) \equiv \max_y \left( \frac{\partial v_x}{\partial x}\bigg|_{x_{par}} \right)$$

When the streamlines are nearly parallel, both of these gradients should be very small. A simple criterion assumes that two infinitesimally-separated points drift apart by an amount set by the maximum velocity gradient. We thus impose a condition of the form,

$$x_{par}^2 \; a(x_{par})/v^{swim} \ll 1$$
$$x_{par}^2 \; b(x_{par})/v^{swim} \ll 1$$

For the best-fit squirmers to the experimental data, $x_{par}$ is several body lengths away from the swimmer.

**Numerical Work.** Because of the sensitivity of chaotic dynamics to numerical instabilities, we perform high-precision simulations of single particles advected by the blinking flow field, rather than direct transport calculations using the advection-diffusion equation. A variable-step integration scheme was applied using Mathematica's built-in NDSolve function. The code produces an ensemble of trajectories $\mathbf{r}_i(t)$ corresponding to single algae particles

with different initial locations advected by the flow.

**Capture calculations**. The density function is approximated from the simulation results as,

$$\rho(\mathbf{r}, t) = \frac{1}{N} \sum_{i=1}^{N} \delta(\mathbf{r} - \mathbf{r}_i(t)) \tag{A1}$$

In general, quantities that depend on the integral of $\rho(\mathbf{r}, t)$ (such as the total capture rate) may be computed efficiently from simulation results by reversing the order of integration and summation—i.e, by performing the integrals first for each numerically computed trajectory.

Because larvae feed via interception, the instantaneous feeding rate of the organism $f_i(t)$ is proportional to the number of particles currently within an interception distance $\delta$ of its surface. For the larval system, $\delta$ is chosen to equal the lengths of single cilia relative to the body radius, $\sim 30\mu m/500\mu m = 0.06$. The total particles in the near field at a given time is computed to be

$$\mathcal{E}(t) = \int_{1}^{1+\delta} \rho(\mathbf{r}, t)\ d\mathbf{r}.$$

We define the ciliary capture rate per unit time for particles within this near field as $\gamma$. For a purely absorptive feeder $\gamma = 1$ and all incident particles are immediately captured, $f_i(t) \propto \mathcal{E}(t)$. This case has been investigated explicitly for the squirmer model in previous theoretical work.[54] In this limit, the surface acts as a sink, and the dynamics of the concentration field must be updated over time to account for particle flux at the boundary.

However, for organisms with ciliary bands, individual captures are rare compared to the number of particles near the surface at a given time, and so we instead work in the limit that the capture rate per unit time is vanishingly small. This limit allows capture dynamics to be computed *ex post facto* from advection simulations, without the need for auxiliary simulation of depletion of the nutrient field. In previous work we have verified that $f$ and $\delta$ are both vanishingly small for the starfish larval system, and that the dependence of particle capture on these two parameters is linear when they are small, due to monotonicity of the capture process.[4] In this limit, $\rho(\mathbf{r}, t)$ has dynamics given primarily by advection, although

a leading-order correction term may be added account for gradual loss of particles due to capture.

In this rare-capture limit, we compute the time-averaged feeding rate $\bar{f}$ for a given swimming strategy by performing long numerical simulations containing multiple blinks,

$$\bar{f} = \gamma \lim_{t \to \infty} \left( \frac{1}{t} \int_0^t \int_0^{2\pi} \int_a^{a+\delta} \rho(\mathbf{r}, t') \; r dr d\theta dt' \right)$$

Because this quantity scales linearly with the specific small value of $\gamma$ used to determine capture rates, we primarily describe relative values of this averaged feeding rate in the main text.

Using a similar approach, we may also calculate the angular distribution of captured incident particles in the low-capture limit,

$$p(\theta) = \gamma \int_0^\infty \int_1^{1+\delta} \rho(\mathbf{r}, t) \; dr \, dt.$$

Using the raw simulated trajectories, we may also readily compute this quantity for the high-capture limit.

$$p(\theta) = \frac{1}{N} \sum_{i=1}^{N} \int_\infty^\infty \int_1^{1+\delta} \delta(\mathbf{r} - \mathbf{r}_i(t)) \delta(|\mathbf{r}_i(t)| - 1) \delta(t - t_i) \; dr \, dt$$

where $t_i$ is the earliest time at which $|\mathbf{r}_i(t)| = 1$.The second delta function in the integrand ensures that particles are only counted at the location where they first intercept the capture region, and the second delta function prevents multiple-counting of particles that pass in and out of the capture region multiple times. Computationally, this step simply represents a running count of distinct particle trajectories that pass within the annular capture region.

We may also calculate the distribution of incident particles across time, an estimate of

the cumulative number of "capture opportunities" on the surface as a function of time.

$$p(t) = \int_0^{2\pi} \int_1^{1+\delta} \rho(\mathbf{r}, t) \, dr \, d\theta$$

In the low-capture limit, the total particles captured over time scales linearly with the product of this quantity and the instantaneous particle capture rate $\gamma$ determined by the cilia,

$$\bar{f}_{low} = \lim_{t \to \infty} \left( \frac{1}{t} \gamma p(t) \right)$$

In the high-capture limit, we fall back to single particle trajectories to evaluate arrival distributions

$$\bar{f}_{high} = \lim_{t, N \to \infty} \left( \frac{1}{t\,N} \sum_{i=1}^{N} \int_0^{2\pi} \int_1^{1+\delta} \delta(\mathbf{r} - \mathbf{r}_i(t)) \delta(|\mathbf{r}_i(t)| - 1) \delta(t - t_i) \, dr \, d\theta \right)$$

where $t_i$ and the delta functions are defined as above for the individual trajectory simulations. This integral is essentially a running count of the total number of particles that ever enter the near field, divided by the total number of particles simulated.

**Rapid-blink limit, $\mathbf{St}^{-1} \to 0$.** One limiting case occurs when the average period between behavioral switches $T$ is very short relative to the time it takes particles to travel appreciable distances relative to the swimmer's body during a blink of duration $\nu T$ (where $\nu$ is the dimensionless duty cycle). In this case, particles undergo very small relative deflections during a given blink and the motion of particles can be described by a single, "effective" velocity field given by,

$$\mathbf{v}_{eff}(\mathbf{r}) = (1 - \nu) \mathbf{v}_{swim}(\mathbf{r}) + \nu v_{blink}(\mathbf{r}) \tag{A2}$$

The average swimming speed is also a $\nu$ weighted average of the two modes. The mean capture rate may thus be computed from the trajectories of particles subject to this "average" field,

$$\bar{f} = \bar{f}\,[\mathbf{v}_{eff}]$$

We use this calculation to determine the bottom edge of the capture rate vs. $\nu$ vs $T$ plot in the main text.

**Rare-blink limit, $\mathbf{St}^{-1} \to \infty$.** An opposite limiting case occurs if the interval between behavioral switches is large compared to the time it takes particles to travel large distances relative to the swimmer. In this case, the displacement of particles during transitions is a rare enough event that it contributes a negligible amount to the overall capture rate.

In this case, the effective capture rate becomes the weighted average of the separate capture rates under the two swimming modes,

$$\bar{f} = (1-\nu)\bar{f}_{swim} + \nu \bar{f}_{blink} \tag{A3}$$

where the subscripted quantities are calculated using simulations of the two flow fields under steady conditions. This limit applies to organisms that cannot easily change their behavioral states, and it suggests that whichever single swimming stroke produces the highest instantaneous feeding rate will also produce the highest overall feeding rate. For the squirmer model, the optimal feeding rate in a homogenous environment occurs when the swimming speed is maximized, as has been found for explicit numerical studies that couple the squirmer model to the advection-diffusion equation.[54]

**Intermediate values of $\mathbf{St}^{-1}$.** The two limits described above implicitly suggest that organisms with the ability to modulate their swimming strokes should do it often enough that it affects their average feeding rate a meaningful amount, but not so often that particles undergo negligible displacements from their streamlines. This intermediate regime is where streamline crossing and other transient and timescale dependent effects become particularly relevant to the feeding strategy, and it also comprises the circumstances under which chaotic advection becomes possible. For this region, we perform long numerical simulations with a fixed-length algae cloud, as the two parameter $\nu$ and $\mathrm{St}^{-1}$ are varied. We then use the capture rate in the small $f$ limit computed above in order to estimate the relative feeding

rate associated with each set of timescale parameters.
